# Supplementary material for: Generation of 3D Brain MRI Using Auto-Encoding Generative Adversarial Networks
Source: arXiv:1908.02498 source file (2019-08-07)
Supplement: Supplementary file 1 [file paper1635-supp_compressed_fin.pdf]

# Supplementary Material

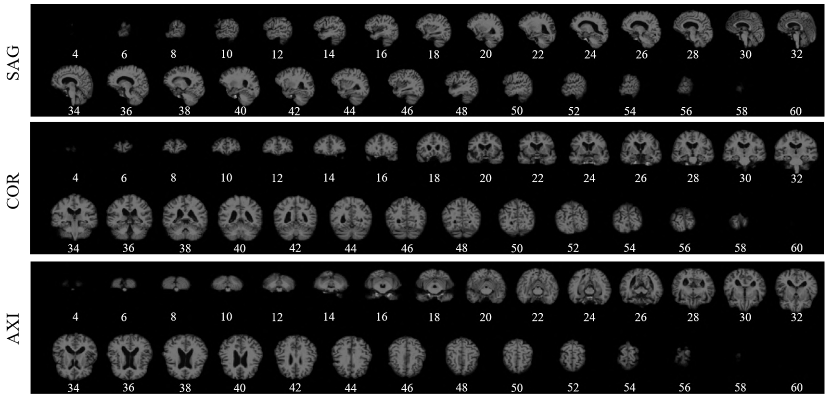


(a) Real

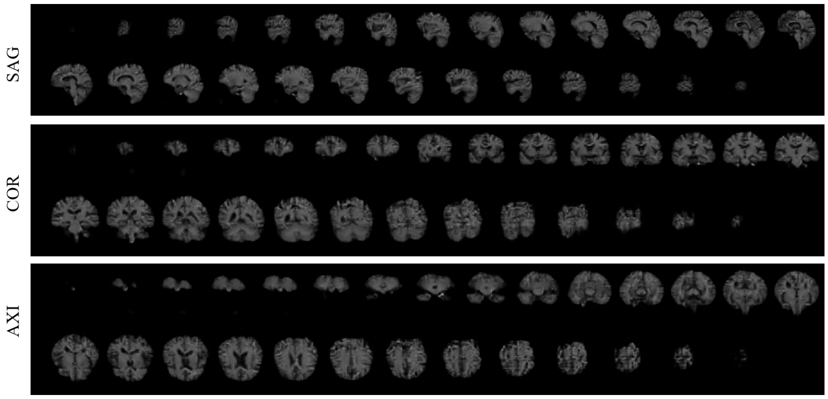


(b) Ours

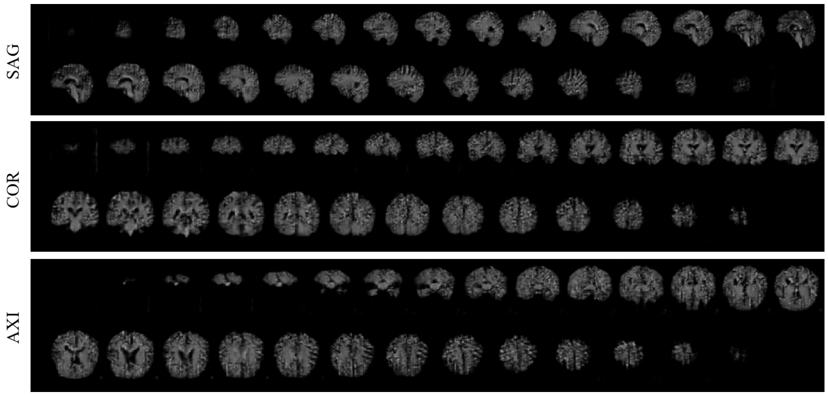


(c) 3D-$\alpha$-GAN

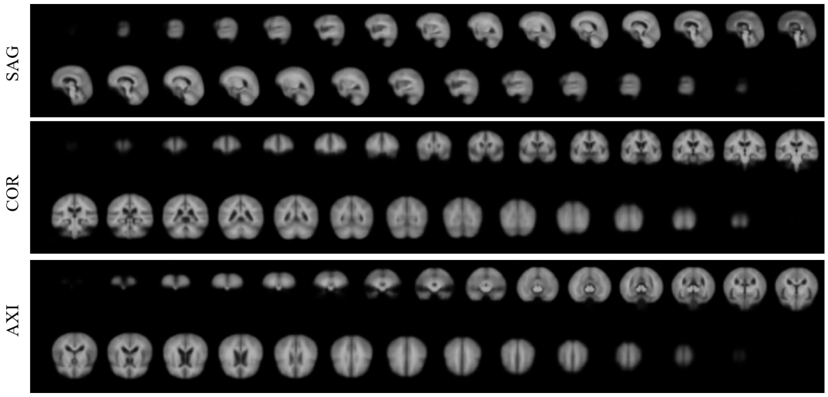


(d) 3D-VAE-GAN

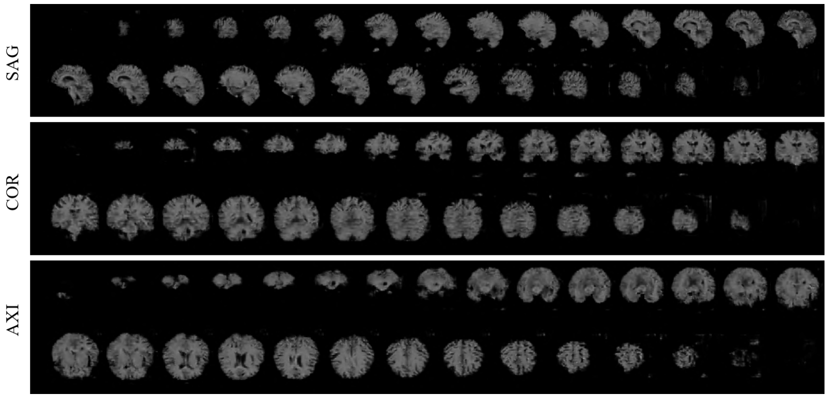


(e) 3D-WGAN-GP

Fig. 1: Slices of normal brain 3D samples from (a) real data, (b) Ours, (c) 3D-$\alpha$-GAN, (d) 3D-VAE-GAN, (e) 3D-WGAN-GP, along sagittal (SAG), coronal (COR) and axial (AXI) planes. The numbers below the images indicate slice numbers.

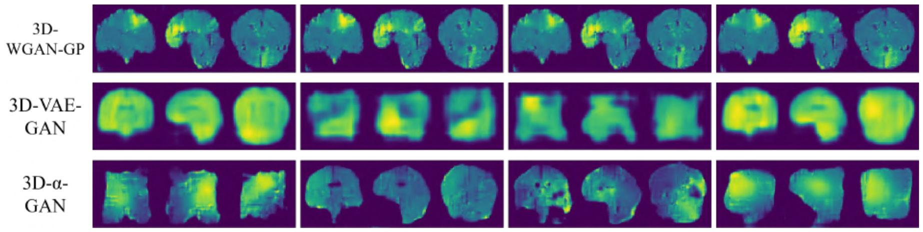


(a) Tumor-FLAIR

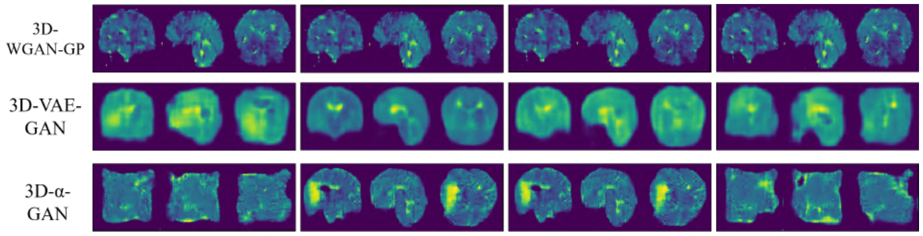


(b) Tumor-T2

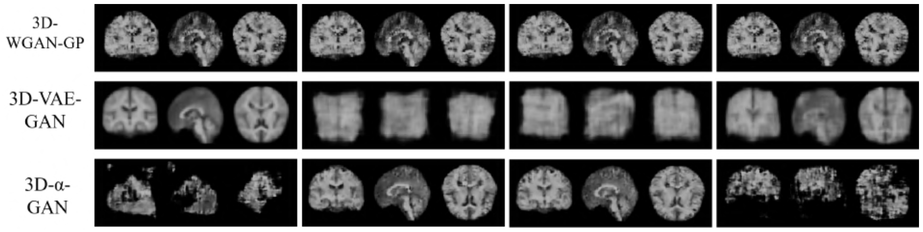


(c) Stroke-T1w

Fig. 2: Generated center-cut views of diseased brain samples from baseline models. For 3D-$\alpha$-GAN and 3D-VAE-GAN, samples are severely deteriorated. 3D-WGAN-GP suffers from mode collapse generating samples with little variance.

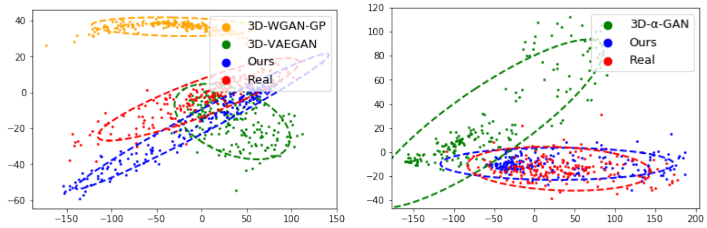


(a) Tumor-FLAIR

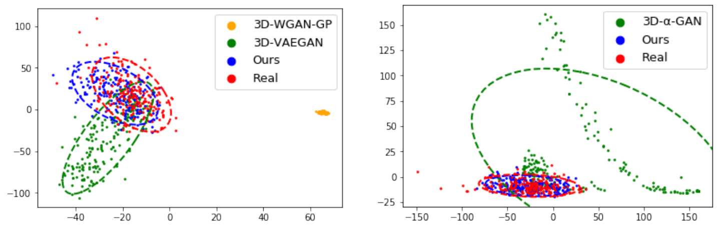


(b) Tumor-T2

Fig. 3: PCA results of generated tumor brain samples. (a) Tumor-FLAIR Samples from real data, baseline models, and Ours. (b) Tumor-T2 Samples from real data, baseline models, and Ours. Samples from our model have the closest distribution to the real data.

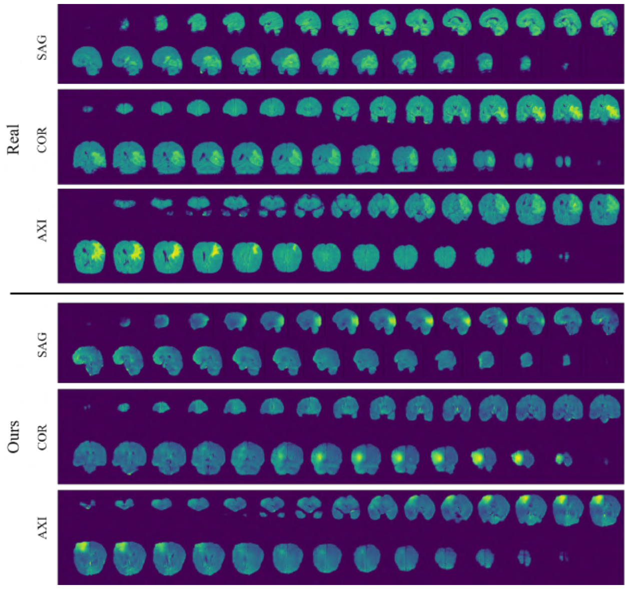


Fig. 4: Slices of tumor-FLAIR brain 3D samples from real data and our model along sagittal (SAG), coronal (COR), and axial (AXI) planes.

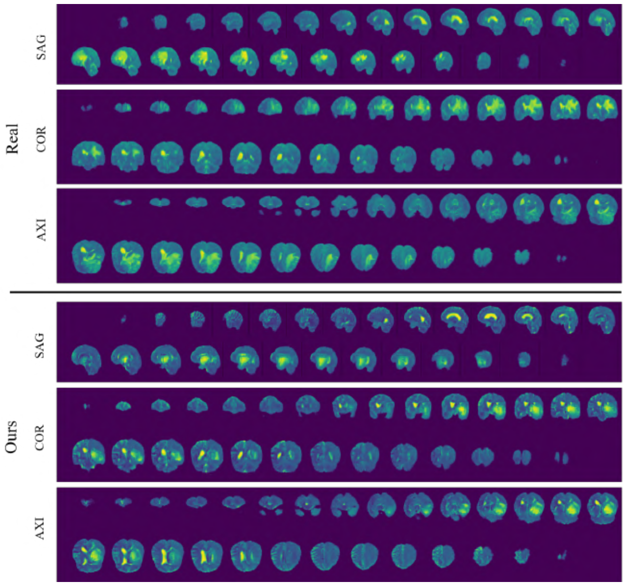


Fig. 5: Slices of tumor-T2 brain 3D samples from real data and our model along sagittal (SAG), coronal (COR), and axial (AXI) planes.

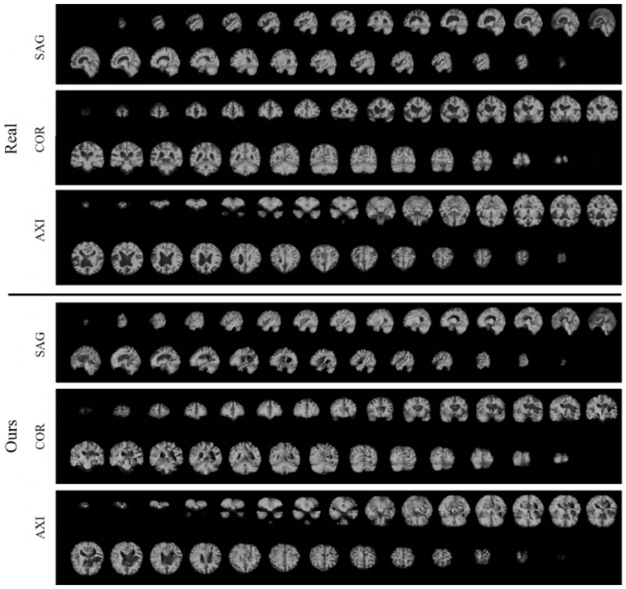


Fig. 6: Slices of stroke-T1w brain 3D samples from real data and our model along sagittal (SAG), coronal (COR), and axial (AXI) planes.
